# Supplementary material for: Analyzing the Real-World Applicability of DGA Classifiers
Source: arXiv:2006.11103 source file (2020-06-19)
Supplement: Supplementary file 1 [file appendix.tex]

% !TEX root = ../paper.tex
\section{Appendix}
\label{sec:appendix}
In Appendix \ref{sec:appendix_statistical_data}, we provide additional statistical data for the binary classification experiments of Section \ref{sec:binary_classification} and the multiclass classification experiments of Section \ref{sec:multiclass_classification}. Appendix~\ref{sec:appendix_mcc_confusion_matrix} includes the confusion matrix of M-ResNet.MI from the multiclass classification experiment in the unbalanced scenario (Section \ref{sec:unbalanced_scenario}). In Appendix \ref{sec:appendix_b_vs_u}, we present the individual TPRs and FNRs of FANCI and B-ResNet per DGA from our analysis of the effect of class imbalance on the binary classification task  (Section~\ref{sec:b_vs_ub}).

\newpage

\subsection{Statistical Data}
\label{sec:appendix_statistical_data}

\begin{table}[!htbp]
	\caption{Binary Classification: Mixed DGAs \newline (Section~\ref{sec:binary_classification_mixed_dga})}
	\label{tab:statistical_values_binary_mixed}
	\centering
	\resizebox{\columnwidth}{!}{
		\begin{tabular}{llccccl}
			\toprule
			\textbf{Classifier} & \textbf{} & \textbf{ACC} & \textbf{TPR} & \textbf{TNR} & \textbf{FNR} & \textbf{FPR} \\
			\midrule
			\multirow{5}{*}{FANCI}& $\overline{x}$ & 0.99764 &	0.99744 & 0.99784 & 0.00256 & 0.00216 \\
			& $\sigma$ & 0.00010 &	0.00013 & 0.00017 & 0.00013 & 0.00017 \\
			& $x_{min}$ & 0.99743 &	0.99714 & 0.99759 & 0.00234 & 0.00164 \\
			& $\tilde{x}$ & 0.99764 &	0.99742 & 0.99780 & 0.00258 & 0.00220 \\
			& $x_{max}$ & 0.99787 &	0.99766 & 0.99836 & 0.00286 & 0.00241 \\
			\midrule
			\multirow{5}{*}{B-Endgame} & $\overline{x}$ & 0.99891 &	0.99969 & 0.99813 &	0.00031 & 0.00187 \\
			& $\sigma$ & 0.00016 &	0.00016 & 0.00028 &	0.00016 & 0.00028 \\
			& $x_{min}$ & 0.99833 &	0.99904 & 0.99703 &	0.00004 & 0.00126 \\
			& $\tilde{x}$ & 0.99893 &	0.99971 & 0.99814 &	0.00029 & 0.00186 \\
			& $x_{max}$ & 0.99926 &	0.99996 & 0.99874 &	0.00096 & 0.00297 \\
			\midrule
			\multirow{5}{*}{B-NYU} & $\overline{x}$ & 0.99907 &	0.99976 & 0.99838 &	0.00024 & 0.00162 \\
			& $\sigma$ & 0.00013 &	0.00013 & 0.00027 &	0.00013 & 0.00027 \\
			& $x_{min}$ & 0.99872 &	0.99933 & 0.99776 &	0.00004 & 0.00102 \\
			& $\tilde{x}$ & 0.99909 &	0.99978 & 0.99837 &	0.00022 & 0.00163 \\
			& $x_{max}$ & 0.99939 &	0.99996 & 0.99898 &	0.00067 & 0.00224 \\
			\midrule
			\multirow{5}{*}{B-ResNet} & $\overline{x}$ & 0.99916 & 0.99978 & 0.99853 &	0.00022 & 0.00147 \\
			& $\sigma$ & 0.00013 &	0.00014 & 0.00024 &	0.00014 & 0.00024 \\
			& $x_{min}$ & 0.99852 &	0.99928 & 0.99739 &	0.00000 & 0.00102 \\
			& $\tilde{x}$ & 0.99917 & 0.99983 & 0.99855 & 0.00017 & 0.00145 \\
			& $x_{max}$ & 0.99938 &	1.00000 & 0.99898 &	0.00072 & 0.00261 \\
			\bottomrule
		\end{tabular}
	}
\end{table}

\begin{table}[!htbp]
	\caption{Binary Classification: Unknown DGAs \newline (Section~\ref{sec:binary_classification_unknown_dga})}
	\label{tab:statistical_values_binary_logo}
	\centering
	\resizebox{\columnwidth}{!}{
		\begin{tabular}{llccccl}
			\toprule
			\textbf{Classifier} & \textbf{} & \textbf{ACC} & \textbf{TPR} & \textbf{TNR} & \textbf{FNR} & \textbf{FPR} \\
			\midrule
			\multirow{5}{*}{FANCI}& $\overline{x}$ & 0.98073 &	0.96392 & 0.99754 &	0.03608 & 0.00246 \\
			& $\sigma$ & 0.00034 &	0.00061 & 0.00027 &	0.00061 & 0.00027 \\
			& $x_{min}$ & 0.97978 &	0.96198 & 0.99696 &	0.03526 & 0.00199 \\
			& $\tilde{x}$ & 0.98077 &	0.96405 & 0.99759 &	0.03595 & 0.00241 \\
			& $x_{max}$ & 0.98131 &	0.96474 & 0.99801 &	0.03802 & 0.00304 \\
			\midrule
			\multirow{5}{*}{B-Endgame} & $\overline{x}$ & 0.98569 &	0.97307 & 0.99830 &	0.02693 & 0.00170 \\
			& $\sigma$ & 0.00272 &	0.00542 & 0.00019 &	0.00542 & 0.00019 \\
			& $x_{min}$ & 0.97945 &	0.96043 & 0.99779 &	0.01516 & 0.00125 \\
			& $\tilde{x}$ & 0.98554 & 0.97269 & 0.99831 & 0.02731 & 0.00169 \\
			& $x_{max}$ & 0.99160 &	0.98484 & 0.99875 &	0.03957 & 0.00221 \\
			\midrule
			\multirow{5}{*}{B-NYU} & $\overline{x}$ & 0.98406 &	0.96961 & 0.99851 &	0.03039 & 0.00149 \\
			& $\sigma$ & 0.00185 &	0.00365 & 0.00018 &	0.00365 & 0.00018 \\
			& $x_{min}$ & 0.97999 &	0.96187 & 0.99806 &	0.02198 & 0.00108 \\
			& $\tilde{x}$ & 0.98421 &	0.96996 & 0.99853 &	0.03004 & 0.00147 \\
			& $x_{max}$ & 0.98841 &	0.97802 & 0.99892 &	0.03813 & 0.00194 \\
			\midrule
			\multirow{5}{*}{B-ResNet} & $\overline{x}$ & 0.98517 &	0.97168 & 0.99866 &	0.02832 & 0.00134 \\
			& $\sigma$ & 0.00153 &	0.00304 & 0.00018 &	0.00304 & 0.00018 \\
			& $x_{min}$ & 0.98054 &	0.96262 & 0.99818 &	0.02337 & 0.00093 \\
			& $\tilde{x}$ & 0.98537 &	0.97204 & 0.99864 &	0.02796 & 0.00136 \\
			& $x_{max}$ & 0.98764 &	0.97663 & 0.99907 &	0.03738 & 0.00182 \\
			\bottomrule
		\end{tabular}
	}
\end{table}

%\subsection{Multiclass Experiments: Statistical Data}
%\label{sec:appendix_mcc}
\begin{table}[!htbp]
	\caption{Multiclass Classification: Balanced Scenario \newline (Section~\ref{sec:balanced_scenario})}
	\label{tab:statistical_values_mcc_balanced}
	\centering
	\tiny
	\resizebox{\columnwidth}{!}{
		\begin{tabular}{llccl}
			\toprule
			\textbf{Classifier} & \textbf{} & \textbf{F1-score} & \textbf{Precision} & \textbf{Recall} \\
			\midrule
			\multirow{5}{*}{M-Endgame}& $\overline{x}$ & 0.86841 & 0.87636 & 0.87028 \\
			& $\sigma$ & 0.00121 & 0.00153 & 0.00100 \\
			& $x_{min}$ & 0.86706 & 0.87429 & 0.86898 \\
			& $\tilde{x}$ & 0.86767 & 0.87700 & 0.87004 \\
			& $x_{max}$ & 0.87024 & 0.87827 & 0.87152 \\
			\midrule
			\multirow{5}{*}{M-NYU} & $\overline{x}$ & 0.85937 & 0.86992 & 0.86266 \\
			& $\sigma$ & 0.00224 & 0.00246 & 0.00227 \\
			& $x_{min}$ & 0.85574 & 0.86631 & 0.85892 \\
			& $\tilde{x}$ & 0.85950 & 0.87018 & 0.86289 \\
			& $x_{max}$ & 0.86190 & 0.87275 & 0.86508 \\
			\midrule
			\multirow{5}{*}{M-ResNet} & $\overline{x}$ & 0.87194 & 0.87930 & 0.87367 \\
			& $\sigma$ & 0.00054 & 0.00117 & 0.00071 \\
			& $x_{min}$ & 0.87125 & 0.87802 & 0.87283 \\
			& $\tilde{x}$ & 0.87223 & 0.87878 & 0.87385 \\
			& $x_{max}$ & 0.87250 & 0.88096 & 0.87454 \\
			\bottomrule
		\end{tabular}
	}
\end{table}
\begin{table}[!htbp]
	\caption{Multiclass Classification: Unbalanced Scenario \newline (Section~\ref{sec:unbalanced_scenario})}
	\label{tab:statistical_values_mcc_unbalanced}
	\centering
	\tiny
	\resizebox{\columnwidth}{!}{
		\begin{tabular}{llccl}
			\toprule
			\textbf{Classifier} & \textbf{} & \textbf{F1-score} & \textbf{Precision} & \textbf{Recall} \\
			\midrule
			\multirow{5}{*}{M-Endgame} & $\overline{x}$ & 0.72541 & 0.74319 & 0.72567 \\
			& $\sigma$ & 0.00891 & 0.01081 & 0.00843 \\
			& $x_{min}$ & 0.71070 & 0.72663 & 0.71183 \\
			& $\tilde{x}$ & 0.72897 & 0.74658 & 0.72997 \\
			& $x_{max}$ & 0.73637 & 0.75874 & 0.73566 \\
			\midrule
			\multirow{5}{*}{M-Endgame.MI} & $\overline{x}$ & 0.74312 & 0.76022 & 0.74499 \\
			& $\sigma$ & 0.00597 & 0.00614 & 0.00577 \\
			& $x_{min}$ & 0.73524 & 0.75233 & 0.73658 \\
			& $\tilde{x}$& 0.74373 & 0.76279 & 0.74662 \\
			& $x_{max}$ & 0.75134 & 0.76883 & 0.75168 \\
			\midrule
			\multirow{5}{*}{M-NYU} & $\overline{x}$ & 0.68913 & 0.71867 & 0.68738 \\
			& $\sigma$ & 0.00670 & 0.00884 & 0.00575 \\
			& $x_{min}$ & 0.67734 & 0.70217 & 0.67675 \\
			& $\tilde{x}$ & 0.68890 & 0.72334 & 0.68824 \\
			& $x_{max}$ & 0.69585 & 0.72667 & 0.69265 \\
			\midrule
			\multirow{5}{*}{M-NYU.MI} & $\overline{x}$ & 0.73832 & 0.76104 & 0.73993 \\
			& $\sigma$ & 0.01112 & 0.01057 & 0.01072 \\
			& $x_{min}$ & 0.72070 & 0.74391 & 0.72346 \\
			& $\tilde{x}$ & 0.73722 & 0.75930 & 0.73810 \\
			& $x_{max}$ & 0.75107 & 0.77374 & 0.75181 \\
			\midrule
			\multirow{5}{*}{M-ResNet} & $\overline{x}$ & 0.78878 & 0.81734 & 0.78850 \\
			& $\sigma$ & 0.00196 & 0.00383 & 0.00206 \\
			& $x_{min}$& 0.78664 & 0.81210 & 0.78578 \\
			& $\tilde{x}$ & 0.78796 & 0.81853 & 0.78895 \\
			& $x_{max}$ & 0.79132 & 0.82221 & 0.79152 \\
			\midrule
			\multirow{5}{*}{M-ResNet.MI} & $\overline{x}$ & 0.79648 & 0.81266 & 0.80306 \\
			& $\sigma$ & 0.00300 & 0.00216 & 0.00297 \\
			& $x_{min}$ & 0.79333 & 0.80994 & 0.79837 \\
			& $\tilde{x}$ & 0.79574 & 0.81199 & 0.80357 \\
			& $x_{max}$ & 0.80094 & 0.81632 & 0.80757 \\
			\bottomrule
		\end{tabular}
	}
\end{table}
\pagebreak

\begin{figure*}[!htbp]
	\subsection{Confusion Matrix: Unbalanced Scenario}
	\label{sec:appendix_mcc_confusion_matrix}
	\centering
	\includegraphics[width=\linewidth]{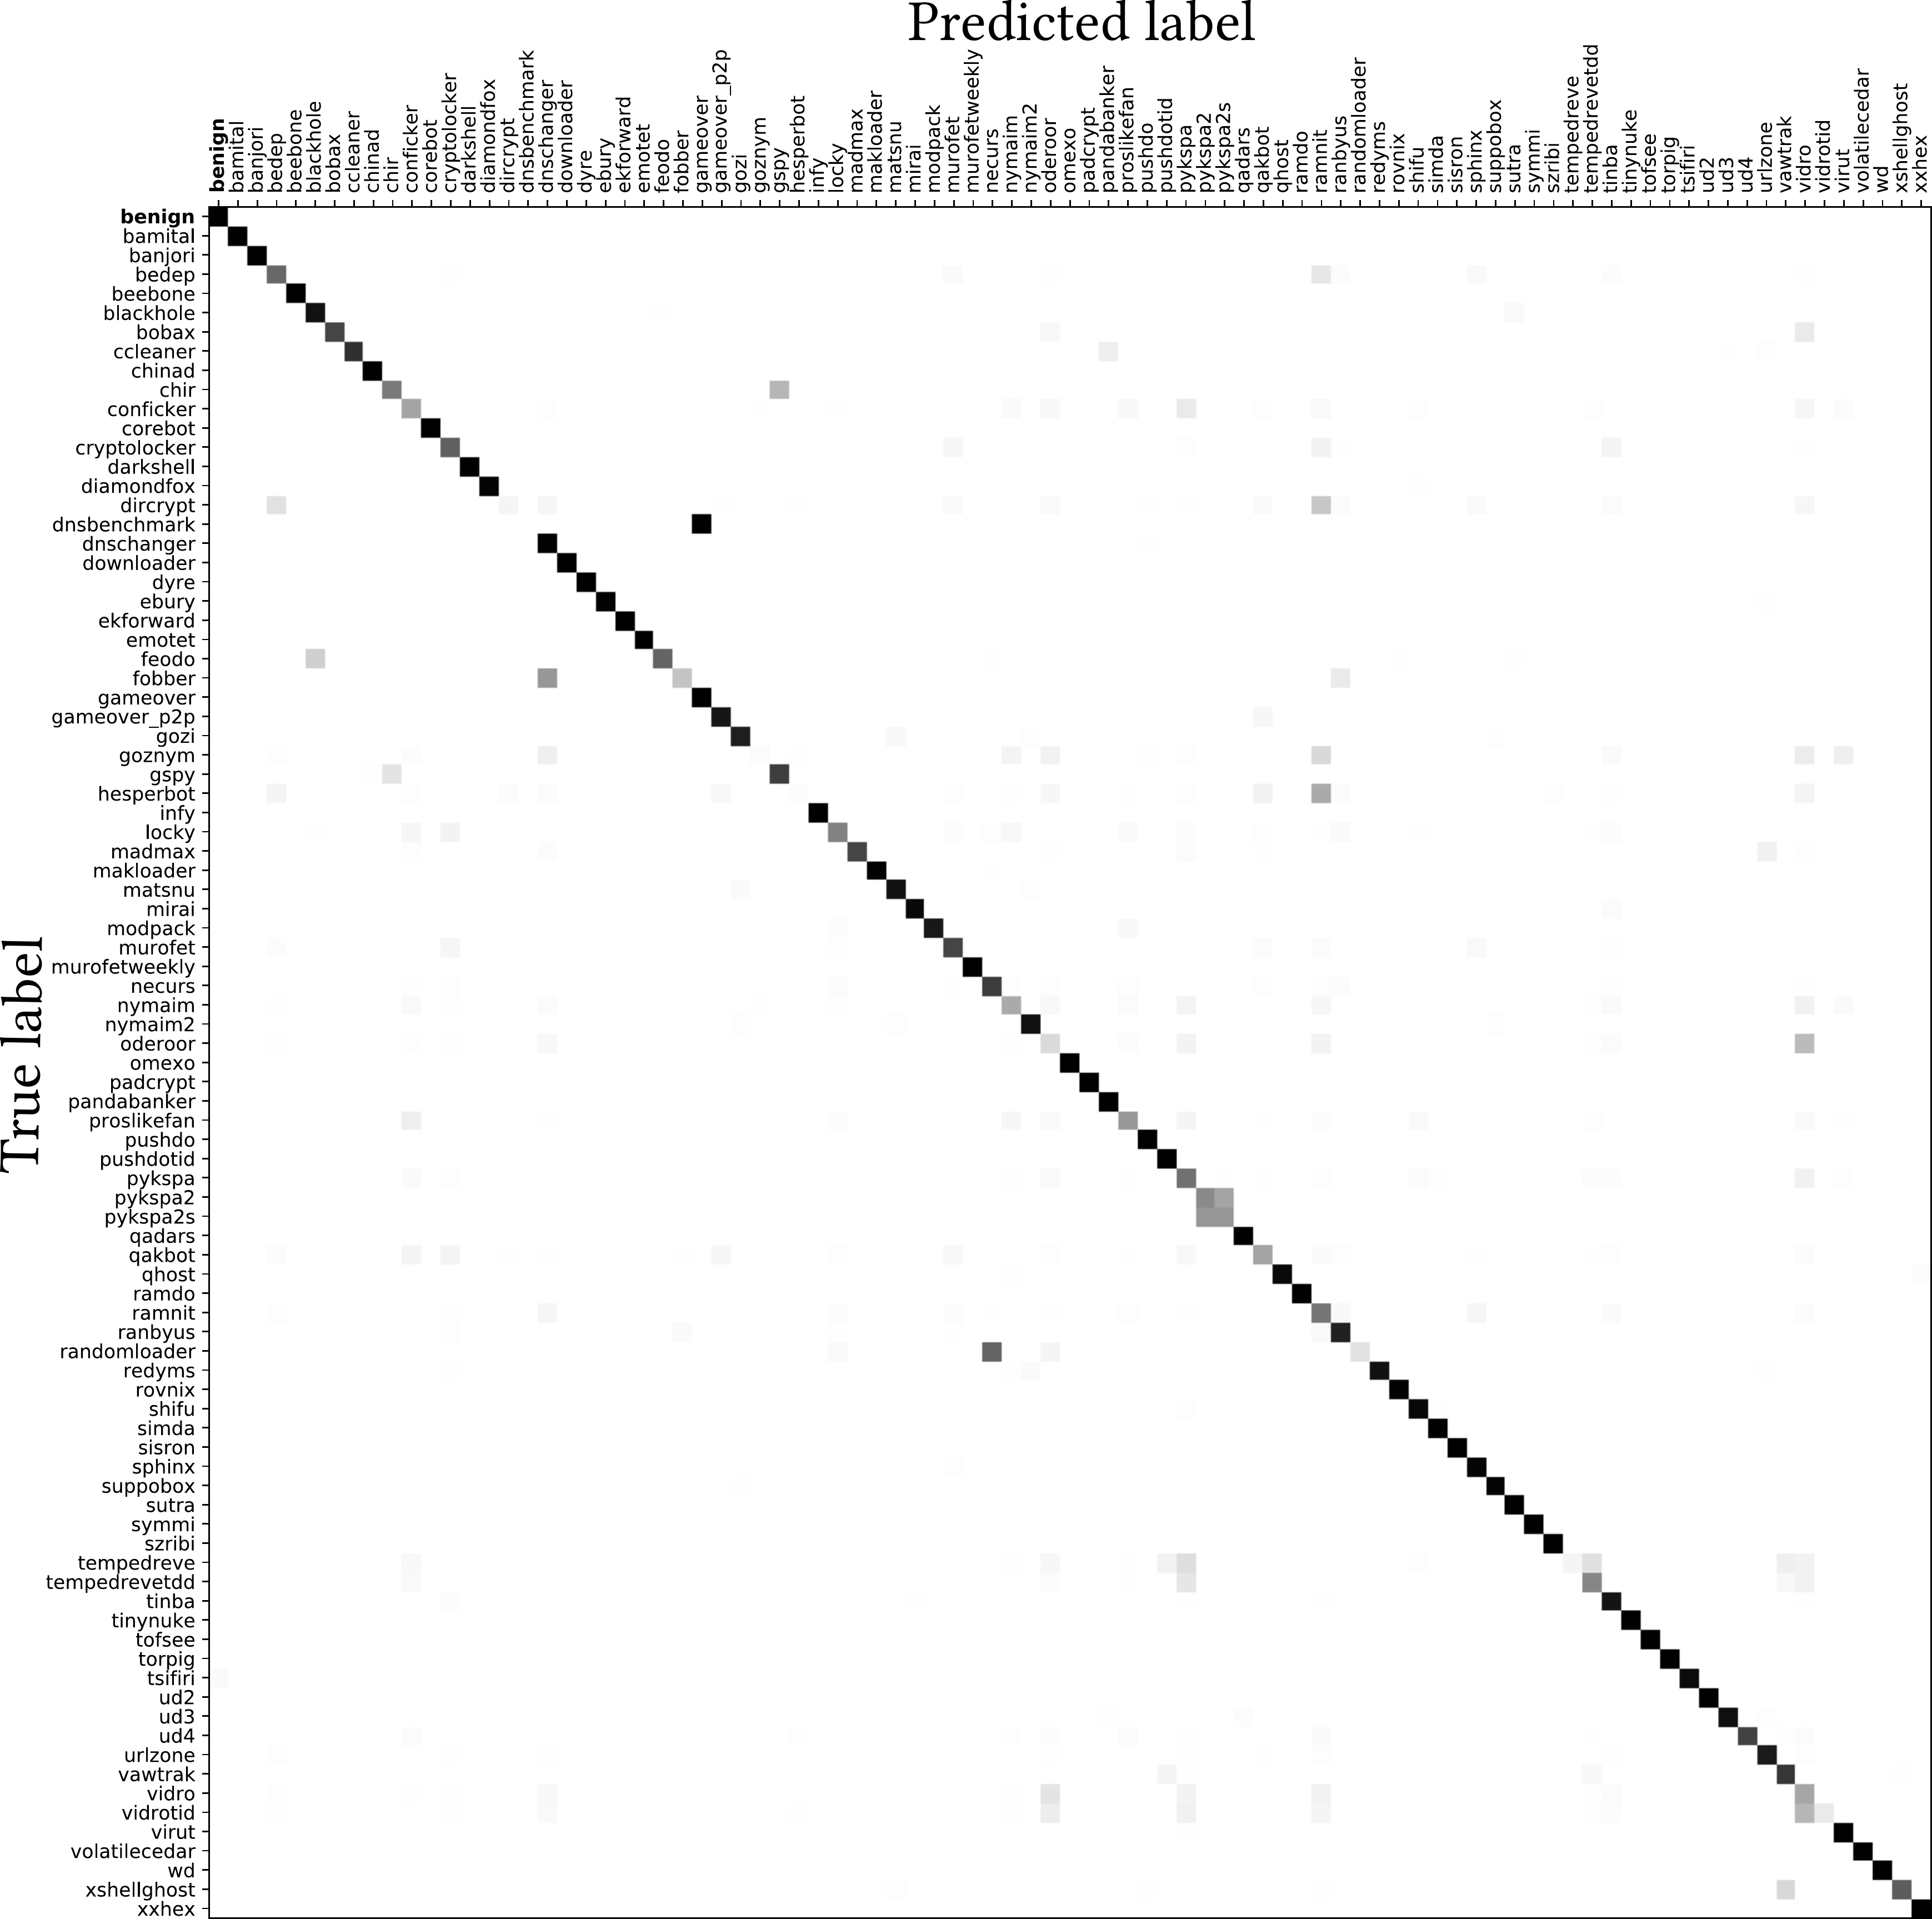}
	\caption{M-ResNet.MI's confusion matrix in the unbalanced scenario (Section \ref{sec:unbalanced_scenario}). The blocks represent the fraction of samples of the classes on the vertical axis which are labeled as classes on the horizontal axis. 100\% is depicted as a clear black block and 0\% is represented by a clear white block.}
	\label{fig:unbalanced}
\end{figure*}

\begin{table*}[!htbp]
	\subsection{Balanced vs. Unbalanced: TPRs/FNRs}
	\label{sec:appendix_b_vs_u}
	\caption{TPRs and FNRs of B-ResNet and FANCI, when trained on B-Balanced-Train and B-Unbalanced-Train, for each individual DGA contained in the B-Unbalanced-Test sets (Section \ref{sec:b_vs_ub}). Improvements of over 1\% of TPR which are achieved by using B-Unbalanced-Train sets are printed in bold. The support denotes the number of samples which are included in the B-Unbalanced-Test sets.}
	\label{tab:b_vs_u_dgas}
	\centering
	\resizebox{\textwidth}{!}{
		\begin{tabular}{lccccccccl}
			\toprule
			\textbf{} & \multicolumn{2}{c}{\textbf{B-ResNet: B-Balanced-Train}} & \multicolumn{2}{c}{\textbf{B-ResNet: B-Unbalanced-Train}} & \multicolumn{2}{c}{\textbf{FANCI:  B-Balanced-Train}} & \multicolumn{2}{c}{\textbf{FANCI:  B-Unbalanced-Train}} & \textbf{} \\
			\textbf{DGA} & \textbf{TPR} & \textbf{FNR} & \textbf{TPR} & \textbf{FNR} & \textbf{TPR} & \textbf{FNR} & \textbf{TPR} & \textbf{FNR} & \textbf{Support} \\
			\midrule
		bedep	        & 1.00000 & 0.00000 & 1.00000 & 0.00000 & 0.99983 & 0.00017 & 0.99986 & 0.00014 & 1492 \\
		\textbf{beebone}	        & \textbf{0.00000} & \textbf{1.00000} & \textbf{1.00000} & \textbf{0.00000} & \textbf{0.00000} & \textbf{1.00000} & \textbf{1.00000} & \textbf{0.00000} & 42 \\
		blackhole	    & 1.00000 & 0.00000 & 1.00000 & 0.00000 & 1.00000 & 0.00000 & 1.00000 & 0.00000 & 147 \\
		\textbf{bobax}	        & \textbf{0.48163} & \textbf{0.51838} & \textbf{0.99167} & \textbf{0.00833} & \textbf{0.23829} & \textbf{0.76171} & \textbf{0.50356} & \textbf{0.49644} & 60 \\
		ccleaner	    & 1.00000 & 0.00000 & 1.00000 & 0.00000 & 1.00000 & 0.00000 & 1.00000 & 0.00000 & 6 \\
		chir	        & 1.00000 & 0.00000 & 1.00000 & 0.00000 & 1.00000 & 0.00000 & 1.00000 & 0.00000 & 20 \\
		\textbf{darkshell}	    & 1.00000 & 0.00000 & 1.00000 & 0.00000 & \textbf{0.09650} & \textbf{0.90350} & \textbf{0.98977} & \textbf{0.01023} & 10 \\
		\textbf{diamondfox}	    & 0.99961 & 0.00039 & 1.00000 & 0.00000 & \textbf{0.61240} & \textbf{0.38760} & \textbf{0.99938} & \textbf{ 0.00062} & 102 \\
		dircrypt	    & 1.00000 & 0.00000 & 1.00000 & 0.00000 & 1.00000 & 0.00000 & 1.00000 & 0.00000 & 138 \\
		dnsbenchmark	& 1.00000 & 0.00000 & 1.00000 & 0.00000 & 1.00000 & 0.00000 & 1.00000 & 0.00000 & 1 \\
		\textbf{downloader}	    & \textbf{0.00000} & \textbf{1.00000} & \textbf{1.00000} & \textbf{0.00000} & \textbf{0.75000} & \textbf{0.25000} & \textbf{1.00000} & \textbf{0.00000} & 12 \\
		ebury	        & 1.00000 & 0.00000 & 1.00000 & 0.00000 & 0.99996 & 0.00004 & 1.00000 & 0.00000 & 400 \\
		\textbf{ekforward}	    & 0.99778 & 0.00222 & 0.99984 & 0.00016 & \textbf{0.97126} & \textbf{0.02874} & \textbf{0.99985} & \textbf{0.00015} & 607 \\
		feodo	        & 1.00000 & 0.00000 & 1.00000 & 0.00000 & 1.00000 & 0.00000 & 1.00000 & 0.00000 & 39 \\
		fobber	        & 0.99998 & 0.00002 & 1.00000 & 0.00000 & 1.00000 & 0.00000 & 1.00000 & 0.00000 & 400 \\
		goznym	        & 1.00000 & 0.00000 & 1.00000 & 0.00000 & 1.00000 & 0.00000 & 1.00000 & 0.00000 & 73 \\
		gspy	        & 1.00000 & 0.00000 & 1.00000 & 0.00000 & 1.00000 & 0.00000 & 1.00000 & 0.00000 & 10 \\
		hesperbot	    & 1.00000 & 0.00000 & 1.00000 & 0.00000 & 1.00000 & 0.00000 & 1.00000 & 0.00000 & 36 \\
		\textbf{madmax}	        & \textbf{ 0.49810} & \textbf{0.50190} & \textbf{0.96548} & \textbf{0.03452} & \textbf{0.49571} & \textbf{0.50429} & \textbf{0.97351} & \textbf{0.02649} & 84 \\
		makloader	    & 0.99917 & 0.00083 & 1.00000 & 0.00000 & 0.99352 & 0.00648 & 1.00000 & 0.00000 & 103 \\
		\textbf{mirai}	        & \textbf{0.58670} & \textbf{0.41330} & \textbf{1.00000} & \textbf{0.00000} & 0.99661 & 0.00339 & 0.99732 & 0.00268 & 56 \\
		\textbf{modpack}	        & 1.00000 & 0.00000 & 1.00000 & 0.00000 & \textbf{0.79489} & \textbf{0.20511} & \textbf{0.98440} & \textbf{0.01560} & 22 \\
		omexo	        & 1.00000 & 0.00000 & 1.00000 & 0.00000 & 1.00000 & 0.00000 & 1.00000 & 0.00000 & 4 \\
		pushdotid	    & 1.00000 & 0.00000 & 1.00000 & 0.00000 & 0.99994 & 0.00006 & 1.00000 & 0.00000 & 1200 \\
		pykspa2s	    & 1.00000 & 0.00000 & 1.00000 & 0.00000 & 0.99992 & 0.00008 & 0.99992 & 0.00008 & 1992 \\
		\textbf{qhost}	        & 0.99600 & 0.00400 & 1.00000 & 0.00000 & \textbf{0.63200} & \textbf{0.36800} & \textbf{0.99500} & \textbf{0.00500} & 5 \\
		ramdo	        & 1.00000 & 0.00000 & 1.00000 & 0.00000 & 0.99978 & 0.00022 & 0.99988 & 0.00013 & 1200 \\
		randomloader	& 0.99250 & 0.00750 & 1.00000 & 0.00000 & 1.00000 & 0.00000 & 1.00000 & 0.00000 & 1 \\
		redyms	        & 0.99679 & 0.00321 & 1.00000 & 0.00000 & 0.99393 & 0.00607 & 0.99805 & 0.00195 & 7 \\
		shifu	        & 1.00000 & 0.00000 & 1.00000 & 0.00000 & 0.99968 & 0.00032 & 1.00000 & 0.00000 & 467 \\
		sisron	        & 1.00000 & 0.00000 & 1.00000 & 0.00000 & 0.99865 & 0.00135 & 1.00000 & 0.00000 & 1856 \\
		\textbf{sutra}	        & \textbf{0.70786} & \textbf{0.29214} & \textbf{1.00000} & \textbf{0.00000} & \textbf{0.66418} & \textbf{0.33582} & \textbf{0.99896} & \textbf{0.00104} & 1977 \\
		tempedreve	    & 1.00000 & 0.00000 & 1.00000 & 0.00000 & 1.00000 & 0.00000 & 1.00000 & 0.00000 & 41 \\
		tempedrevetdd	& 0.99998 & 0.00002 & 1.00000 & 0.00000 & 1.00000 & 0.00000 & 1.00000 & 0.00000 & 299 \\
		tofsee	        & 0.99857 & 0.00143 & 1.00000 & 0.00000 & 0.99496 & 0.00504 & 1.00000 & 0.00000 & 696 \\
		\textbf{tsifiri}	        & \textbf{0.00000} & \textbf{1.00000} & \textbf{1.00000} & \textbf{ 0.00000} & \textbf{0.03333} & \textbf{0.96667} & \textbf{1.00000} & \textbf{0.00000} & 12 \\
		\textbf{ud2}	            & 1.00000 & 0.00000 & 1.00000 & 0.00000 & \textbf{0.98711} & \textbf{0.01289} & \textbf{1.00000} & \textbf{0.00000} & 83 \\
		\textbf{ud3}	            & \textbf{0.95625} & \textbf{0.04375} & \textbf{0.99583} & \textbf{0.00417} & 0.99188 & 0.00813 & 1.00000 & 0.00000 & 12 \\
		ud4	            & 1.00000 & 0.00000 & 1.00000 & 0.00000 & 1.00000 & 0.00000 & 1.00000 & 0.00000 & 14 \\
		vawtrak	        & 1.00000 & 0.00000 & 0.99991 & 0.00009 & 0.99985 & 0.00015 & 0.99995 & 0.00005 & 540 \\
		vidrotid	    & 1.00000 & 0.00000 & 1.00000 & 0.00000 & 1.00000 & 0.00000 & 1.00000 & 0.00000 & 60 \\
		volatilecedar	& 1.00000 & 0.00000 & 1.00000 & 0.00000 & 1.00000 & 0.00000 & 1.00000 & 0.00000 & 100 \\
		xshellghost	    & 1.00000 & 0.00000 & 1.00000 & 0.00000 & 1.00000 & 0.00000 & 1.00000 & 0.00000 & 11 \\
		\textbf{xxhex}	        & 0.99163 & 0.00837 & 0.99994 & 0.00006 & \textbf{0.95876} & \textbf{0.04124} & \textbf{1.00000} & \textbf{0.00000} & 880 \\
		\midrule
		\textbf{Average}	        & \textbf{0.89097} & \textbf{0.10903} & \textbf{0.99892} & \textbf{0.00108} & \textbf{0.86825} & \textbf{0.13175} & \textbf{0.98726} & \textbf{0.01274} & - \\
		\bottomrule
	\end{tabular}
}
\end{table*}
